# Supplementary material for: Motion Tracking with Muscles: Predictive Control of a Parametric Musculoskeletal Canine Model
Source: arXiv:2506.23768 source file (2026-05-29)
Supplement: Supplementary file 1 [file appendices.tex]

\section
